# Supplementary material for: Polynomial 2D Biharmonic Coordinates for High-order Cages
Source: arXiv:2501.15279 source file (2025-01-25)
Supplement: Supplementary file 1 [file appendix.tex]

\section{Summery of LinearShell}
 \tr{~\cite{Jiang2020BijectivePI} introduces an algorithm to convert a self-intersection free, orientable, and manifold triangle mesh T into a generalized prismatic shell equipped with a bijective projection operator to map T to a class of discrete surfaces contained within the shell whose normals satisfy a simple local condition. Properties can be robustly and efficiently transferred between these surfaces using the prismatic layer as a common parametrization domain. The combination of the prismatic shell construction and corresponding projection operator is a robust building block readily usable in many downstream applications, including the solution of PDEs, displacement maps synthesis, Boolean operations, tetrahedral meshing, geometric textures, and nested cages.}
\section{Proof for Proposition \ref{prop:bezier-curve}}\label{sec:appendix-bezier-curve}
\begin{proof}
    We substitute the control points from equations (\ref{equ:edge-control-1}) to determine the value of the \Bezier curve $\mr(t)$ at a given parameter $t$. This yields the following results:

For equation (\ref{equ:edge-control-1}), the value of $\mr(t)$ is given by:
\begin{equation}\label{equ::param-curve1}
\mr(t)=(1-t) \mx_1+t \mx_2+t (3\beta(1-t)+l t)((1-t)\md_1+t\md_2),
\end{equation}
indicating that $\mr(t)$ is situated on the bilinear patch.

%For equation (\ref{equ:edge-control-2}), $\mr(t)$ is expressed as:
%\begin{equation}\label{equ::param-curve2}
%\mr(t)=\mr_1(t)+(3 \beta-1)t (t-1)\mn_1(t),
%\end{equation}
%where $\mr_1(t)=(1-t)\mx_1+t\mx_2 + \beta t((1-t)\md_1+ t\md_2)$ and $\mn_1(t)=(\mx_1+l t \md_1-(\mx_2+ l t \md_2))$. Here, $\mr_1(t)$ resides on the bilinear patch and $\mn_1(t)$ represents the direction of the isoparametric line of the patch on $\mr(t)$, which shows that $\mr(t)$ is situated on the bilinear patch.

Actually, (\ref{equ::param-curve1}) is the image of the bilinear isoparametric transformation $f(t,s)=(1-s)((1-t)\mx_1+t \mx_2)+s((1-t)(\mx_1+\mn_1)+t(\mx_2+\mn_2))$ on the curve $(t,para_1(t))$, where $para_1(t)=0 t^2+\frac{3\beta}{2} 2t(1-t)+l t^2$.

When it comes to an order 3 \Bezier curve $(t,\beta_1 t(1-t)^2+\beta_2 t^2(1-t)+l t^3)$ on the domain, we have:
$$\mP_1=\mv_1+l \md_1,\mP_5=\mv_2+l \md_2,$$
$$\mP_2=\frac{1}{4}(3\mv_1+\mv_2 +3(l+\beta_1) \md_1+l \md_2),$$
$$\mP_3=\frac{1}{2}(\mv_1+\mv_2+l(\md_1+\md_2)+\beta_1 \md_2+\beta_2 \md_1),$$
$$\mP_4=\frac{1}{4}(\mv_1+3\mv_2+l \md_1+3(l+\beta_2)\md_2)$$

\end{proof}
% \begin{proof}
% 	We substitute the control points in (\ref{equ:edge-control-1}) and (\ref{equ:edge-control-2}) to find the value of the \Bezier curve $\mr(t)$at the parameter $t$, resulting in:

%  for (\ref{equ:edge-control-1}):
%  $$\mr(t)=(1-t) \mx_1+t \mx_2+t (3\beta(1-t)+l t)((1-t)\md_1+t\md_2),$$
%  which shows that $\mr(t)$ lies on the bilinear patch.
 
%  for (\ref{equ:edge-control-2}):
%  $$\mr(t)=r_1(t)+(3 \beta-1)t (t-1)n_1(t),$$
%  where $\mr_1(t)=(1-t)\mx_1+t\mx_2 + \beta t((1-t)\md_1+ t\md_2) $ and $\mn_1(t)=(\mx_1+l t \md_1-(\mx_2+ l t \md_2))$. $\mr_1(t)$ lies on the bilinear patch and $\mn_1(t)$ is the direction of the isoparametric line of the patch on $\mr_(t)$. 
% \end{proof} 

\section{Proof for Proposition \ref{prop:mid2topbase}}\label{sec:appendix-mid2topbase}
\begin{proof}
We only prove the top due to the symmetry.
 We suppose $\hat{t}=\frac{\epsilon_1^{+}}{\|\md_1\|_2},l=\frac{\epsilon_2^{+}}{\|\md_2\|_2}-\frac{\epsilon_1^{+}}{\|\md_1\|_2}, \mp_{\text{mid},2}=\frac{2}{3}\mv_1+\frac{1}{3}\mv_2+\beta \md_1,\mp_{\text{mid},3}=\frac{1}{3}\mv_1+\frac{2}{3}\mv_2+\beta \md_2$. Then we have:
 \begin{equation*}
     \mP_{\text{top},1}=\mx_1,\mp_{\text{top},4}=\mx_2+l \md_2.
 \end{equation*}
 and
 \begin{equation*}
     \mP_{\text{top},2}=\frac{2}{3}\mx_1+\frac{1}{3}\mx_2+\beta_1 \md_1,\mp_{\text{top},3}=\frac{1}{3}\mx_1+\frac{2}{3}\mx_2+\beta_1 \md_1+l \md_1,
 \end{equation*}
 where $\beta_1=\beta+\frac{1}{3}(l+2 \hat{t})$.
 According to Proposition~\ref{prop:bezier-curve}, $\mr_{\text{top}}(t)$ lies on the bilinear surface.
 
 To Calculate $\mr_{\text{top}}(t)-\mr_{\text{middle}}(t)$, we first substitude the control points from Proposition~\ref{prop:mid2topbase} and simplyfy to obtain:
 $$\mr_\text{top}(t) - \mr_\text{middle}(t) = (\frac{\epsilon_1^{+}}{\|\md_1\|_2}(1-t)+\frac{\epsilon_2^{+}}{\|\md_2\|_2}t)((1-t)\md_1 + t\md_2).$$
\end{proof} 

\section{Proof for Proposition \ref{prop:bijective}}\label{sec:appendix-bijective}
\begin{proof}
	%In ~\cite{Jiang2020BijectivePI}, they prove that the isoparametric transformation of prismatic finite element ~\cite{Ciarlet1991BasicEE} is bijective if the volumes of 24 tetrahedra corresponding to 6 tetrahedral decompositions are positive.
	
	Consider the prismatic finite element with six vertices $e_0,e_1,e_2,n_0,n_1,n_2$. The map is defined as:
	\[
	f(u,v,w) = ue_1 + ve_2 + w\eta_0 + uw\eta_1 + vw\eta_2.
	\]
	We denote the Jacobian determinant of $f$ as $J$.
    
	We first give the sufficient \tr{and necessary} condition for this prismatic finite element to be bijective.
	
	\paragraph{Lemma1}The following propositions are equivalent:
	\begin{enumerate}
		\item The prismatic finite element is bijective.
		\item \tr{There do not exists $w\in[0,1]$, such that for three pillars, there exist line corresponding $w$ on the oppisite patch, the line either is parallel or intersecting with the line of the pillar.}
		\item \tr{The adjust patches are not tangent on the pillars, and the lines of pillars do not intersect with the oppisite patch. }
	\end{enumerate}

	\begin{proof}
	\tr{According to ~\cite{Knabner2001TheIO}, the (1)(2)(3) are equal. We first prove (4) is necessary. The adjust patches are tangent shows that $\frac{\partial f}{\partial u}$ $\frac{\partial f}{\partial v}$ are coplanar with the pillar, which is $\frac{\partial f}{\partial w}$. This shows that $J(p)=0$, violate with the bijective condition. It is similiar to the intersection case.}
	
	\tr{We then prove (4) is sufficient. Suppose there is a point $p$ on the pillar such that $J(p)=0$. We have $\frac{\partial f}{\partial u}$ and $\frac{\partial f}{\partial v}$ and $\frac{\partial f}{\partial w}$ are coplanar. If $\frac{\partial f}{\partial u}$ and $\frac{\partial f}{\partial v}$ are on the two sides of $\frac{\partial f}{\partial w}$, then we have the lines of pillars intersect with the oppisite patch. If $\frac{\partial f}{\partial u}$ and $\frac{\partial f}{\partial v}$ are in the same side of $\frac{\partial f}{\partial w}$, then the adjust patches are tangent.}

   \end{proof}
We now turn to the proof of Proposition \ref{prop:bijective}. According to the Lemma1, we have proved that $f$ is bijective on the three pillars (here we suppose $l=0$. If $l\neq 0$, we set $l=max{l_1,l_2,l_3}$, which equal to the case of $l=0$. ). 

\tr{We first prove $f$ is bijective on the trimmed bilinear patches. To be general, we consider the patch $f(u,0,w)$. Since for $u=0,u=1$ the two pillar, $f$ is bijective. we suppose there exist a $t$ such that $f$ is not bijective between $f(t,0,w)$ and $f(1-t,0,w)$. $J$ is continous so there must be a point $p$ on $f(t,0,w)$ or $f(1-t,0,w)$ such that $J(p)=0$. Given $J$ is linear on fixed $w$, $p$ must be on the boundary of top or bottom \Bezier triagnles. Then we have $\frac{\partial f}{\partial u}$ and $\frac{\partial f}{\partial v}$ are coplanar with $\frac{\partial f}{\partial w}$. Then the tangent plane of the \Bezier triangle at $p$ is parallel to $\frac{\partial f}{\partial w}$, i.e. the vector fields, which condradict with the angle condition.}

\tr{With the boundary patches are bijective, it is similiar to prove $f$ is bijective on the whole shell space. The point $p$ such that $J(p)=0$ must be on the top or bottom bezier triangles, which controdict with the angle condition.}

\end{proof} 

\section{Proof for Proposition \ref{prop:projection}}\label{sec:appendix-projection}
\begin{proof}
Since the vector field can be regarded as the isoparametric transformation $\mf$ on a prism $\tilde{\triangle}$. $\tilde{\triangle}$ is obtained by extending the unit prism $\hat{\triangle}$ along the z-axis in space, where $\hat{\triangle}=\{u, v \geq 0 | u+v \leq 1\} \times [-1, 1]$, identifying the bottom surface of \( \hat{\Lambda} \) as \( z = -1 \), middle surface as \( z = 0 \), and top surface as \( z = 1 \).
We consider the inverse of the isoparametric transformation. 
Since the isoparametric transformation is bijective, $\mf^{-1}$ is bijective. 
In particular, $\mf^{-1}$ transforms $\cF$ to the constant vector \( \mathbf{e}_z = (0, 0, 1) \). 
The projection operator can thus be equivalently defined as $ Proj(p) = \mf^{-1}(P_{\tilde{\triangle}}(\mf(p))$, where \( P_{\tilde{\triangle}} \) is the projection over the \( z \)-axis in the reference prism. 
\( P_{\tilde{\triangle}} \) is bijective if the piecewise linear mesh intersecting \( \triangle \) is composed of triangles with positive area (and the boundaries are mapped to the boundaries), after being mapped to the reference \( \tilde{\triangle} \) and projected by \( P_{\tilde{\triangle}} \).
In the reference domain, having a positive area after projection (with a fixed boundary) is equivalent to that the dot product between the projection direction and the normal of every face is positive.
	\end{proof}

\section{Proof for Proposition \ref{prop:vector-query}}\label{sec:appendix-vector-query}
\begin{proof}
	Since $\cP$ satisfies the bijective condition, we can find $v$ within $\mt_{\text{linear}}$ s.t. $\md(\mv) = u_1 \md_1+u_2 \md_2+ u_3 \md_3$ hit $\mp$, which shows that there exit a real root $t$ of the cubic equation in accordance with the given proposition. If we can find another $\tilde{v}$ within $\mt_{\text{linear}}$, then $\cF$ is not injective at $\mp$, contradicting our conditions.

 Due to the symmetry, we next only prove $t_\text{real}$ is the smallest positive real root of the cubic equation if $\left\langle\mv_2-\mv_1,\mv_3-\mv_1,\md-\mv_1\right\rangle>0$. Suppose there is a $\tilde{t}_{\text{real}}>0$ and $\tilde{t}_{\text{real}}<t_{\text{real}}$, we consider the function $a(t)=\left \langle \mp_2-\mp_1,\mp_3-\mp_1,\md(\mv)\right \rangle$, which is a quadratic function related to $t$. We have $a(0)>0,a(t_{\text{real}})=0,a(\tilde{t}_{\text{real}})=0$ , which shows that $a(t)<0$ for $t\in (\tilde{t}_{\text{real}},t_{\text{real}})$. According to Proposition~\ref{prop:bijective}, the isoparametric transformation is not bijective, leading to a contradiction.
\end{proof}
